# Supplementary material for: Towards Transitive-free Digraphs
Source: arXiv:2503.10541 source file (2025-03-13)
Supplement: Supplementary file 1 [file appendix.tex]

\newpage

\section*{{\Large Appendix}}

\section{Extended Preliminaries}\label{Sec:apppreli}

\section{Proof of Claim \ref{clm:bounded}} \label{Sec:bddproof}
